# Supplementary material for: Watch Me, but Don't Touch Me! Contactless Control Flow Monitoring via Electromagnetic Emanations
Source: arXiv:1708.09099 source file (2017-08-30)
Supplement: Supplementary file 1 [file sec-appendix.tex]

\appendix \label{sec:appendix}

%\begin{scriptsize}
%\begin{verbatim}
%\end{verbatim}
%\end{scriptsize}

this is the appendix
% \input{Sources/subsec-implementation}

\begin{comment}

\begin{figure*} [tp]
\centering
\begin{subfigure}[tp]{0.33\textwidth}
  \includegraphics[scale=0.33]{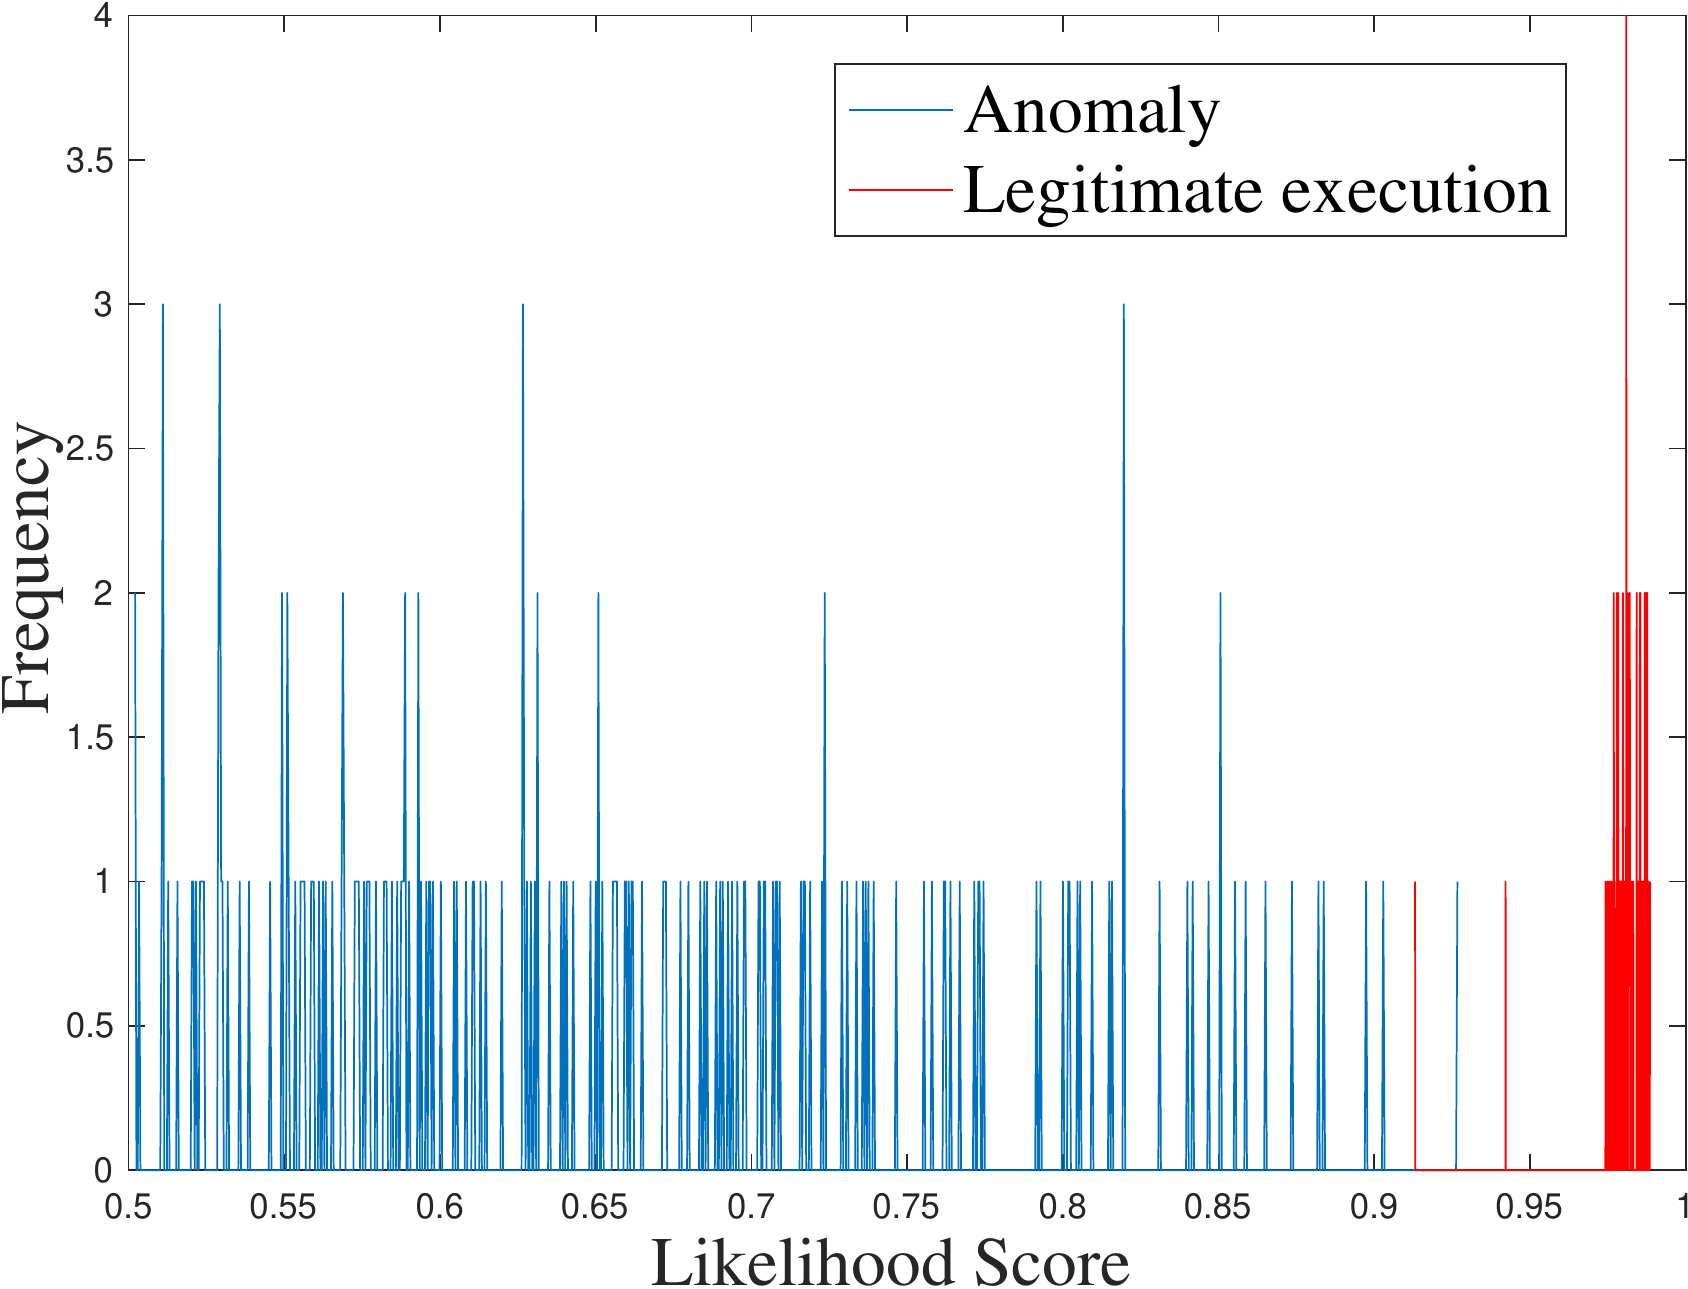}
  \caption{mat}
  \label{fig:likedistmat}
\end{subfigure}
%
\begin{subfigure}[tp]{0.33\textwidth}
  \includegraphics[scale=0.33]{conv}
  \caption{new}
  \label{fig:likedistnew}
\end{subfigure}
%
\begin{subfigure}[tp]{0.33\textwidth}
  \includegraphics[scale=0.33]{conv}
  \caption{gd}
  \label{fig:likedistgd}
\end{subfigure}
\begin{subfigure}[tp]{0.33\textwidth}
  \includegraphics[scale=0.33]{conv}
  \caption{qsort}
  \label{fig:likedistqsort}
\end{subfigure}
%
\begin{subfigure}[tp]{0.33\textwidth}
  \includegraphics[scale=0.33]{conv}
  \caption{dct}
  \label{fig:likedistdct}
\end{subfigure}
%
\begin{subfigure}[tp]{0.33\textwidth}
  \includegraphics[scale=0.33]{conv}
  \caption{conv}
  \label{fig:likedistconv}
\end{subfigure}
%
\begin{subfigure}[tp]{0.33\textwidth}
  \includegraphics[scale=0.33]{conv}
  \caption{aes}
  \label{fig:likedistaes}
\end{subfigure}
%
\begin{subfigure}[tp]{0.33\textwidth}
  \includegraphics[scale=0.33]{conv}
  \caption{pid}
  \label{fig:likedistpid}
\end{subfigure}
%
\begin{subfigure}[tp]{0.33\textwidth}
  \includegraphics[scale=0.33]{conv}
  \caption{patfilt}
  \label{fig:likedistpatfilt}
\end{subfigure}
%
\begin{subfigure}[tp]{0.33\textwidth}
  \includegraphics[scale=0.33]{conv}
  \caption{cod}
  \label{fig:likedistcod}
\end{subfigure}

\end{comment}
